# Supplementary material for: Preventing Catastrophic Overfitting in Fast Adversarial Training: A Bi-level Optimization Perspective
Source: arXiv:2407.12443 source file (2024-07-17)
Supplement: Supplementary file 2 [file supp.tex]

We present the relationship between the classification accuracy and training time of the comparison AT algorithms shown in Fig.~\ref{perform}.
\begin{figure}[htbp]
	\centering
	\includegraphics[width=0.5\linewidth]{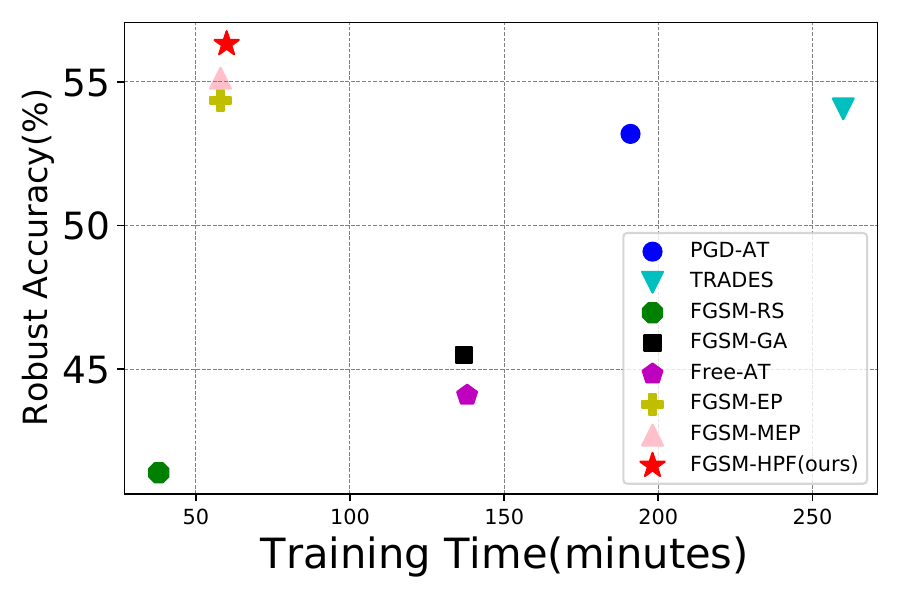}
	\caption{Relationship between the classification accuracy under PGD10 attack and training time on the ResNet18 with the CIFAR10 dataset.}
	\label{perform}
\end{figure}
